# Supplementary material for: Multi-modal Situated Reasoning in 3D Scenes
Source: arXiv:2409.02389 source file (2024-11-18)
Supplement: Supplementary file 1 [file MSR3D_additional_qualitative_results_crop.pdf]

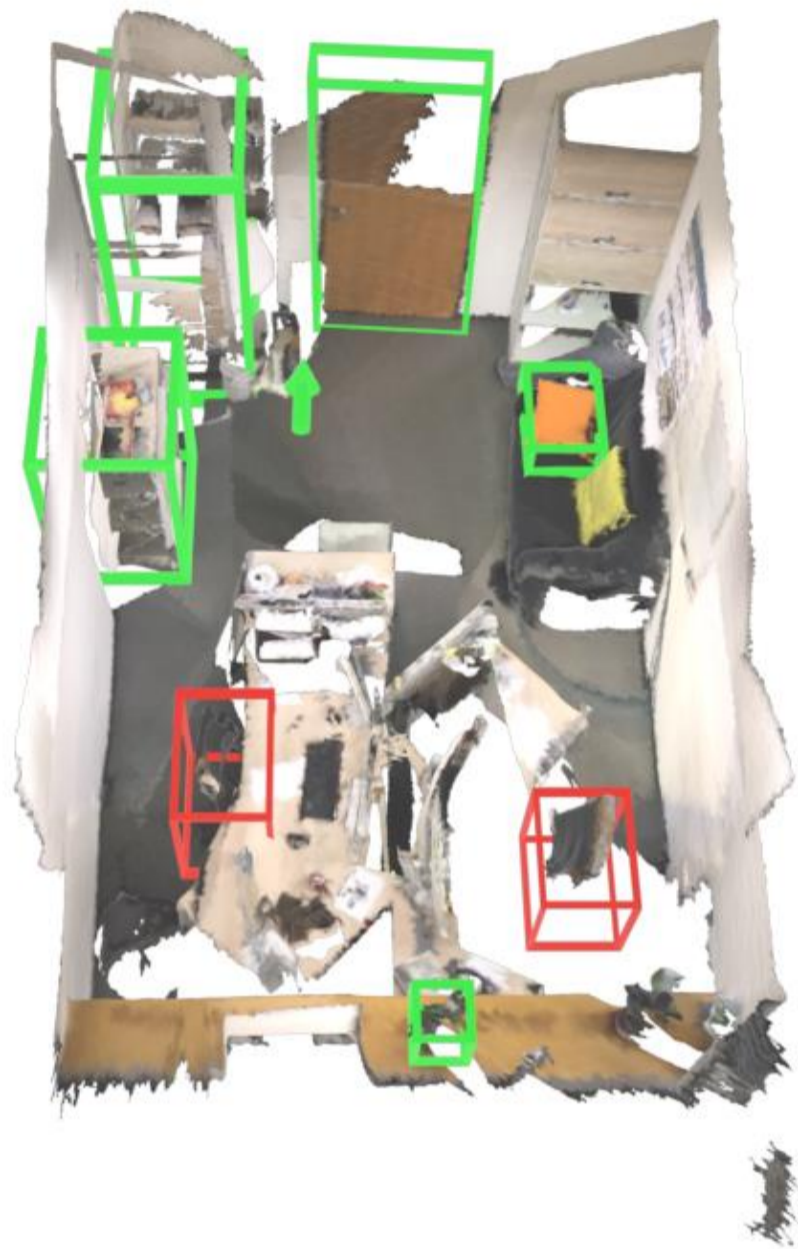

a)

### Situation:

There is an orange pillow at my 3 o'clock direction, a

brown

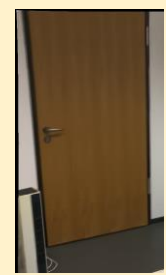

at my 1 o'clock direction, and a white

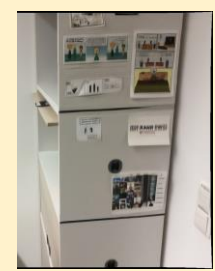

at my 9 o'clock direction. In front of me, at a

middle distance, there's a gray metal

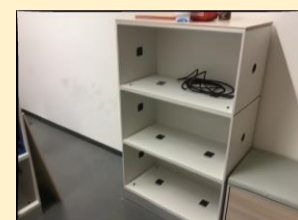

and a

me, there is

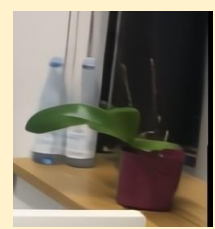

.

**Question:** In which direction from me is the object used for seating?

**MSR3D:** at your 5 o'clock

**GPT-4o:** The object used for seating is located at your 2 o'clock and 8 o'clock directions (for the couch and one chair), another chair is in front of you (at around 12 o'clock direction).

**Ground truth:** at your 7 o'clock

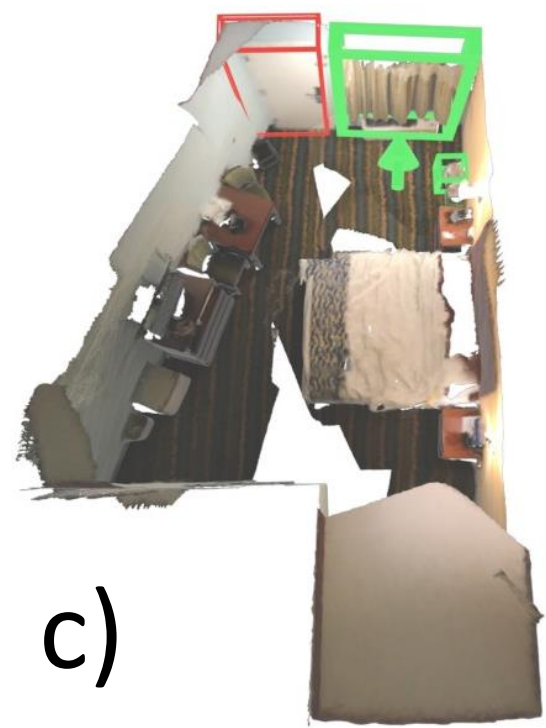

c)

**Situation:** I am closing the curtain. To my right, near me, there's a semi-transparent white bag.

**Question:** How many doors are at my 9 o'clock?

**MSR3D :**one

**GPT-4o:** There are no doors at your 9 o'clock.

**Ground truth:** one

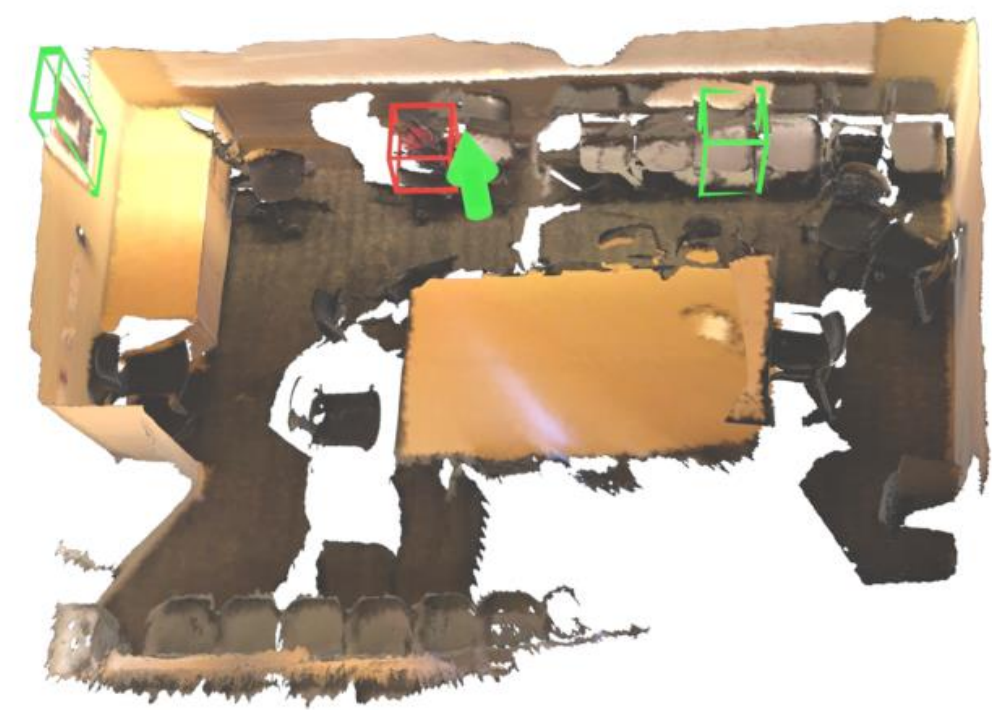

b)

### Situation:

There is a brown

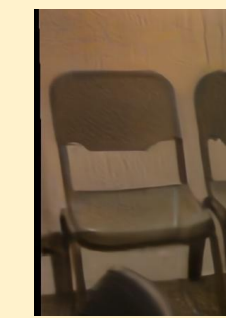

made of plastic at my 3

o'clock direction. A black and white

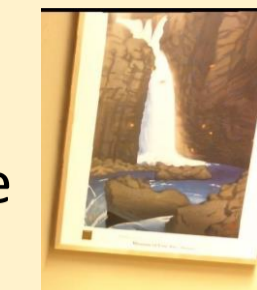

is at my 9

**Question:** What object is used for carrying items at my 11 o'clock?

**MSR3D:** the backpack

**GPT-4o:** The object used for carrying items at your 11 o'clock is a red backpack.

**Ground truth:** the backpack

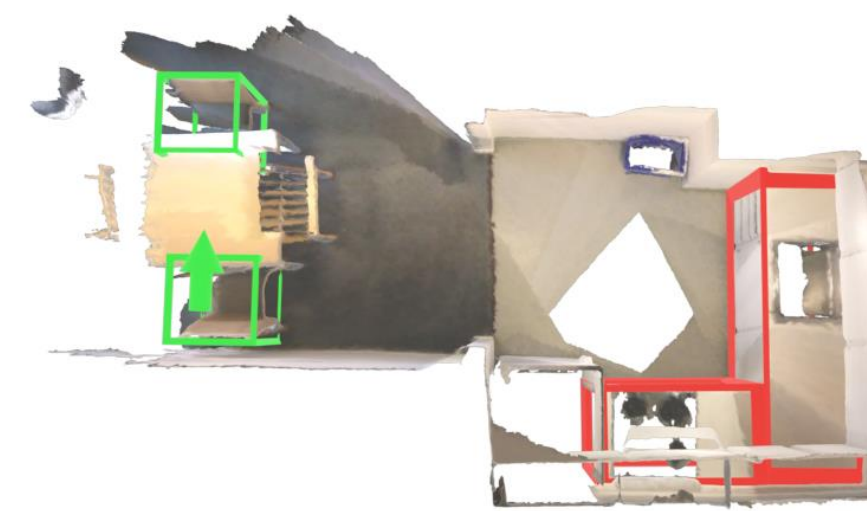

d)

### Situation:

I am sitting on the

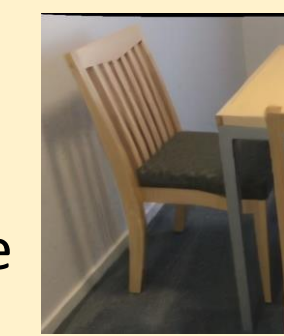

. In front of me, near,

there's a light brown and black

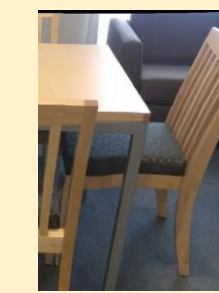

in use.

**Question:** How many kitchen cabinets are in the far distance on my right?

**MSR3D:** two

**GPT-4o:** There are two kitchen cabinets in the far distance on your right.

**Ground truth:** two

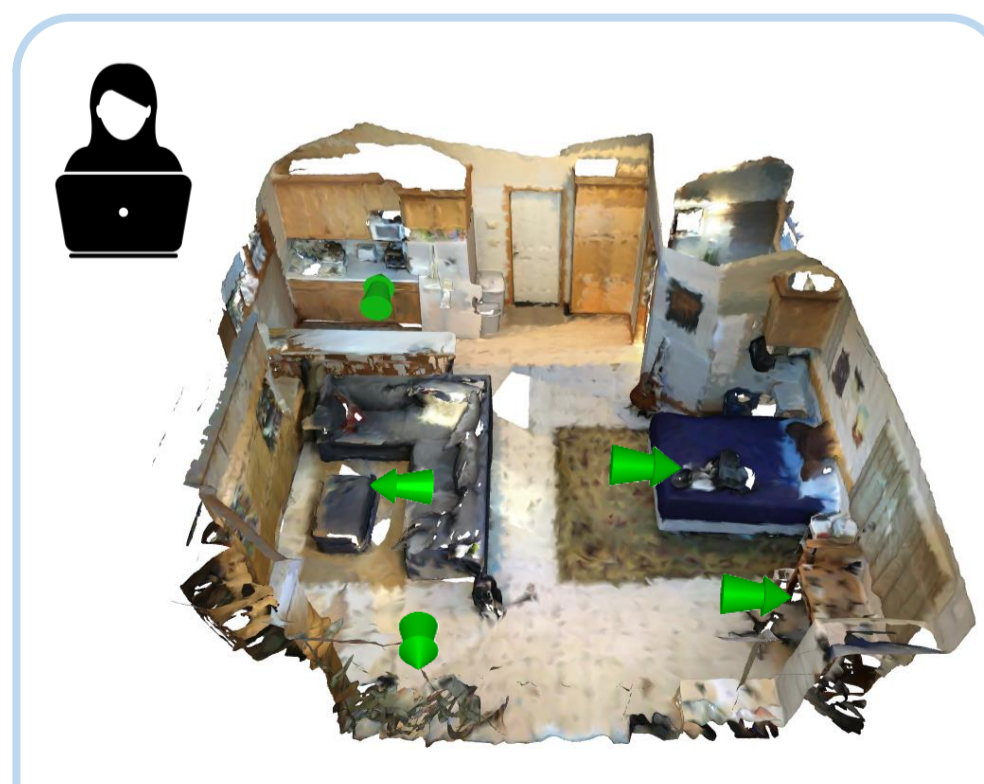

### I. Situation Identification

Participants are asked to pick  $\langle s^{\text{pos}}, s^{\text{rot}} \rangle$  and write description  $s^{\text{txt}}$ .

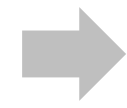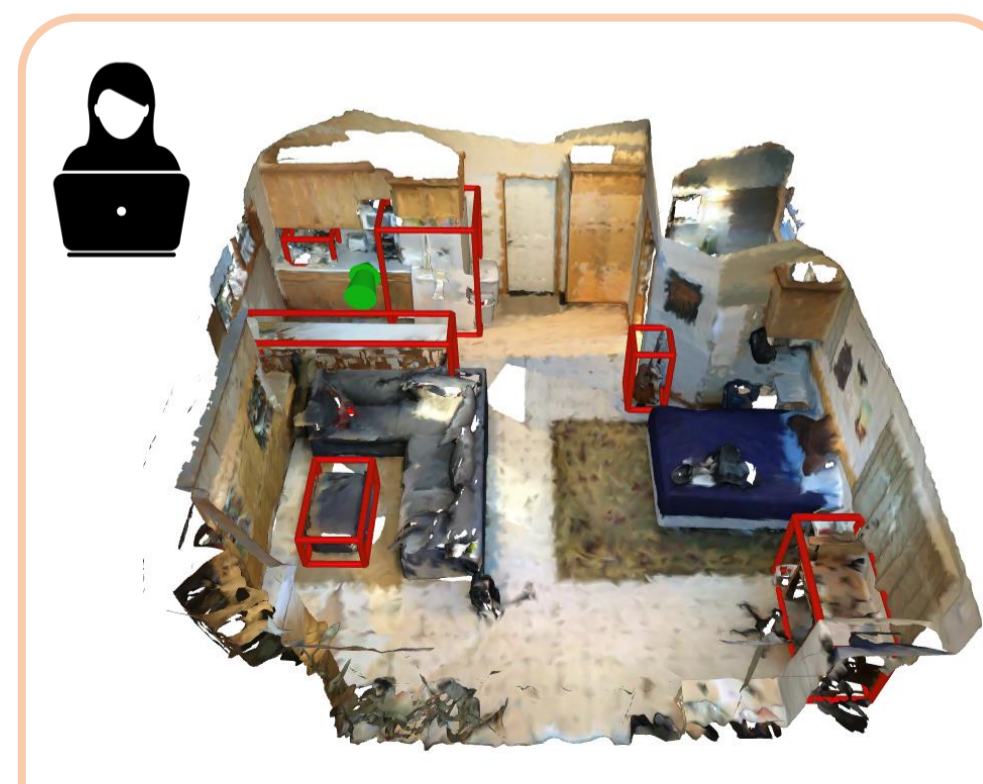

### II. Question Preparation

Participants are asked to write question  $q$  given the situation depicted in both  $\langle s^{\text{pos}}, s^{\text{rot}} \rangle$  and  $s^{\text{txt}}$ .

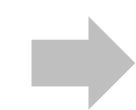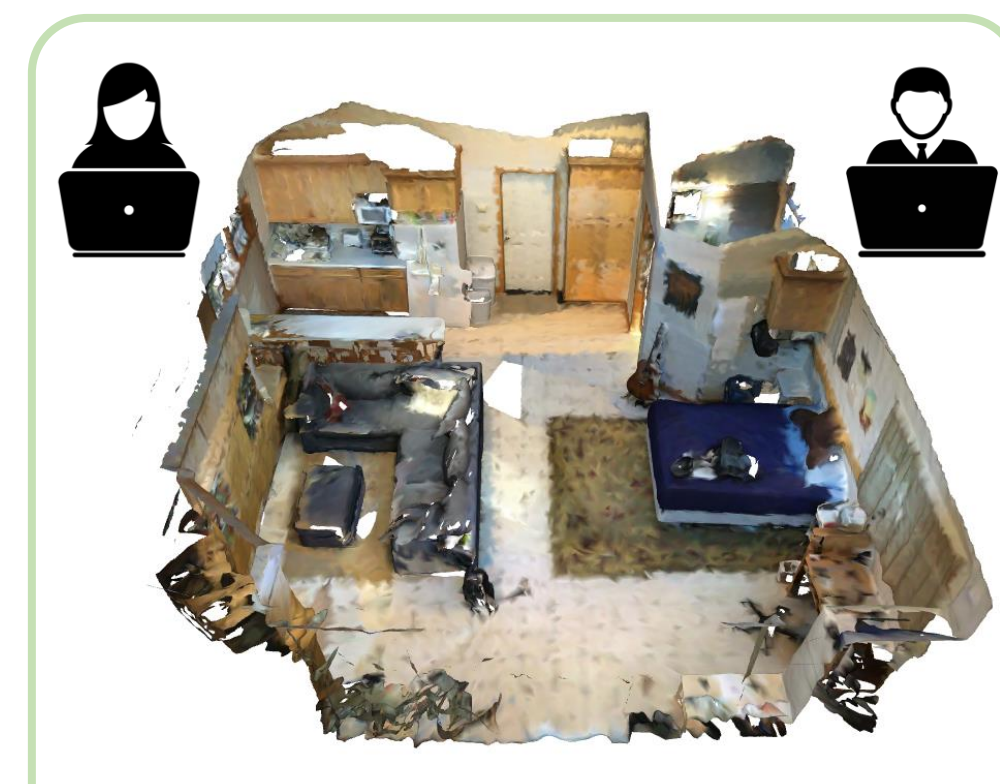

### III. Answer Collection & Human Study

More participants are asked to answer question  $q$  given the situation depicted **only** in  $s^{\text{txt}}$ .
